# Supplementary material for: Static and dynamic friction in sliding colloidal monolayers
Source: arXiv:1208.4856 ancillary file (2012-08-29)
Supplement: Supplementary file 1 [file supporting_information_PNAS_vanossi_manini_tosatti_2012.pdf]

*Supporting Information*

# Static and dynamic friction in sliding colloidal monolayers

Andrea Vanossi, Nicola Manini, and Erio Tosatti

(Dated: August 18, 2012)

## I. MODEL DETAILS

We describe colloidal particles as classical point-like objects moving under the action of external forces, the mutual repulsion, and the interaction with the viscous solution in which they are immersed.

The equation of motion for the $j$-th particle is:

$$m\ddot{\mathbf{r}}_j + \eta(\dot{\mathbf{r}}_j - v_d\hat{\mathbf{x}}) = -\nabla_{\mathbf{r}_j}(U_2 + U_{\rm ext}), \qquad (1)$$

where $\mathbf{r}_j$ is a 2-dimensional displacement vector relative to the center of the cell, and $v_d$ is the drift velocity, giving rise to the Stokes' driving force $F = \eta v_d$, experienced by all the colloidal particles.

For the slow motion ($v_d\ 1\mu ms^-1$) of a colloidal particle in the liquid the inertial term can be neglected, and a diffusive motion can safely be assumed, with an appropriate choice of $\eta$ (given in Table II). Thermal (Brownian) motion is easily simulated by adding suitable random Gaussian forces in a Langevin approach, but, after verifying that thermal effect are small at 300 K, we mostly consider $T = 0$ deterministic equations, which offer neater pictures of the same physics.

The 2-body interaction is

$$U_2 = \sum_{j<j'}^{N} V(|\mathbf{r}_j - \mathbf{r}'_j|) \qquad (2)$$

and the screened Coulomb repulsion varies with interparticle distance as a Yukawa-type potential

$$V(r) = \frac{Q}{r}\exp(-r/\lambda_D)\,. \qquad (3)$$

The above expression holds only for separation $r$ larger than the diameter $\simeq$ 3.9 $\mu$m of a colloidal particle, where an additional hard-core repulsion sets in. Typical nearest-neighbor experimental colloid separations are $r \simeq 5.7$ nm $\simeq 30\lambda_D$ [1]. Colloids rarely approach very closely, for the violent increase of Coulomb repulsion in $V(r)$ keeps them apart well before the hard-core repulsion sets in. Explicit inclusion of the hard-core term is thus unnecessary as it would cause no change in the colloid trajectories. Given the moderate volume fraction occupied by the colloidal particles in the solution and the adiabatically slow motions under study, it is also appropriate to neglect hydrodynamic forces [2], that would become relevant only at much denser/faster regimes.

The 1-body external potential energy

$$U_{\rm ext} = \sum_{j}^{N} V_{\rm ext}(\mathbf{r}_j) \qquad (4)$$

| $n$ | 2 | 3 | 4 | 5 | 6 |
|---|---|---|---|---|---|
| $c_n$ | 1 | 4/3 | $\sqrt{2}$ | 2 | $4/\sqrt{3}$ |
| $\alpha_n$ | 0 | 0 | $\pi/4$ | 0 | $-\pi/6$ |

TABLE I: Values of parameters that generate $\mathbf{k}_l$ of Eq. (8). For $n > 6$, yielding a quasi-periodic symmetry, $c_n = 1$ and $\alpha_n = 0$.

is introduced by a laser field, and can be shaped with substantial freedom. We assume the following spatial variation:

$$V_{\rm ext}(\mathbf{r}) = G(\mathbf{r})[-A_c + U_0\,W_n(\mathbf{r})]\,, \qquad (5)$$

where

$$G(\mathbf{r}) = \exp\left(-\frac{|\mathbf{r}|^2}{2\sigma^2}\right)\,, \qquad (6)$$

is an unnormalized Gaussian of (large) width $\sigma$, accounting for the overall intensity envelope of the laser beam, and

$$W_n(\mathbf{r}) = -\frac{1}{n^2}\left|\sum_{l=0}^{n-1}\exp(i\,\mathbf{k}_l\cdot\mathbf{r})\right|^2\,, \qquad (7)$$

is a periodic (for $n = 2, 3, 4$, or 6) or quasi-periodic potential of $n$-fold symmetry [3] produced by the interference of $n$ laser beams, representing the substrate corrugation. The appropriate 2D interference pattern is realized by taking

$$\mathbf{k}_l = \frac{c_n\pi}{a_{\rm las}}\left[\cos\left(\frac{2\pi l}{n}+\alpha_n\right), \sin\left(\frac{2\pi l}{n}+\alpha_n\right)\right]. \qquad (8)$$

The numerical constants $c_n$ are chosen in order to match the potential lattice spacing to the laser interference periodicity $a_{\rm las}$, and $\alpha_n$ are chosen so that one of the primitive vectors of the periodic potential $W_n(\mathbf{r})$ is directed along the $x$ axis. These numerical coefficients are reported in Table I.

The two positive amplitudes $A_c$ and $U_0$ set respectively the intensity of the overall potential confining the colloids near the simulation-cell center, and the intensity of the corrugated, spatially oscillating term. Note that both of them are controlled by the same overall Gaussian intensity modulation, Eq. (5), consistently with experiment [1]. The simulation is carried out in dimensionless units, defined in terms of the physical quantities of Table II. Our simulated colloid island has a small but not negligible extension compared with the Gaussian width $\sigma$

| physical quantity | model expression | typical value |
|---|---|---|
| length | $a_{\rm coll}$ | 5.7 $\mu$m |
| force | $F_0 = 9F_{s1}/(8\pi)$ | 18 fN |
| viscosity coefficient | $\eta$ | $6.3 \times 10^{-8}$ kg/s |
| energy | $F_0\, a_{\rm coll}$ | $1.0 \times 10^{-19}$ J |
| time | $\eta a_{\rm coll}^2/U_0$ | 20 s |
| mass | $\eta^2 a_{\rm coll}/F_0$ | $1.3 \times 10^{-6}$ kg |
| velocity | $F_0/\eta$ | 0.284 $\mu$m/s |
| power | $F_0^2/\eta$ | $5.1 \times 10^{-21}$ W |

TABLE II: Basic units for various quantities in our model, with typical values appropriate for the setup by Bohlein *et al.* [1].

| | $\eta$ | $N$ | $Q$ | $\lambda_D$ | $A_c$ | $\sigma$ | $n$ | $U_0$ | $L_x$ | $L_y$ |
|---|---|---|---|---|---|---|---|---|---|---|
| cluster | 1.4 | 28861 | $10^{13}$ | 0.03 | 1200 | 1200 | 3 | 0.1 | 500 | 500 |
| bulk | 1.4 | 28080 | $10^{13}$ | 0.03 | 0.0 | 1200 | 3 | 0.1 | 156 | $90\sqrt{3}$ |

TABLE III: Numerical parameters adopted in the simulation, Eqs. (3), (5), (6), and (7), expressed in model units, to be scaled according to Table II. $L_x$ and $L_y$ are the sides of the rectangular simulation supercell respectively.

as shown in Table III. As a result, the colloid pinning effect of the corrugated potential weakens somewhat in the outer region, compared to the central area.

We simulate the colloidal system in a periodically repeated rectangular box of sides $L_x$ and $L_y$ where periodic boundary conditions are implemented for particle-particle interactions, but not for the external potential $V_{\rm ext}(\mathbf{r})$ which originates in the central cell only. This choice of boundary conditions applies to both kinds of situations:

1. With $A_c > 0$, an island of particles is located near the center of a much wider supercell, with few or no particle ever crossing the cell boundary. This differs from experiment only sufficiently far from the center, and as in experiment the average density of particles is established by the balance between the interparticle repulsion and the overall trapping forces.

2. With $A_c = 0$, the supercell is filled with a compact monolayer, and only the oscillating potential, its amplitude multiplied by the Gaussian envelope $G(\mathbf{r})$, is felt by the colloids. In this approach one simulates an essentially infinite system, for which a given average colloid density is fixed.

In either version, by choosing appropriate ratios of the average particle spacing to the periodic laser potential spacing $a_{\rm las}$ one can realize a variety of static superstructures, each with its soliton array and pattern. In the present work we adopt the first approach, simulating a large colloid island, with numerical parameters listed in Table III. Unlike experiments, where the colloid density is finite everywhere, and only has a minor decrease outside the Gaussian attractive radius $\sigma$, in our simulated system the density vanishes at the island edge, which is still inside the Gaussian. The experimental "edge" at $r \simeq \sigma$ is therefore much softer than our island hard edge, where density vanishes. That difference is nonetheless expected to make only a quantitative, but not qualitative, difference to the edge-related creation and annihilation of solitons. We did not choose the second approach, closer to experiment, because it is computationally far more expensive, requiring a cell with many million particles, most of which essentially not involved in the soliton physics near the center. We nevertheless adopt that scheme to simulate the infinite-size "bulk" limit, where the overall colloid density is fixed by periodic boundary conditions. In that case, the supercell size is chosen carefully to produce an overall periodic geometry, both relative to the colloid lattice and to the periodic modulation potential $W_n$.

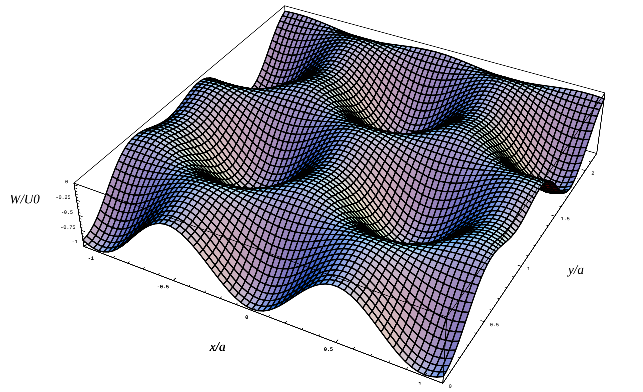


FIG. 1: The triangular-symmetry corrugated potential energy profile $W(x,y) = W_3(x,y)$ as a function of position. Observe the minima at energy $-U_0$, the saddle points at energy $-U_0/9$, and the maxima at energy 0. The resulting lowest energy barrier in the $x$ direction thus equals $\frac{8}{9}U_0$.

As in experiment, we consider a triangular lattice potential, i.e. $n = 3$. The shape of the periodic potential $W(\vec{r}) = W_3(\vec{r})$

$$W(\vec{r}) = -\frac{2}{9}\,U_0\left[\frac{3}{2} + 2\cos\frac{2\pi r_x}{a_{\rm las}}\,\cos\frac{2\pi r_y}{\sqrt{3}a_{\rm las}} + \cos\frac{4\pi r_y}{\sqrt{3}a_{\rm las}}\right] \tag{9}$$

is depicted in Fig. 1. The corrugation profile along $\hat{\mathbf{x}}$, where the barrier is lowest is

$$W(x,0) = -U_0\left(\frac{5}{9} + \frac{4}{9}\cos\frac{2\pi x}{a_{\rm las}}\right), \tag{10}$$

with a barrier amplitude $\frac{8}{9}U_0$. Accordingly, the static friction force for an isolated colloid, i.e. the minimum force that a single colloid requires in order to slide in this one dimensional potential, is

$$F_{s1} = \frac{8\pi U_0}{9a_{\rm las}} = \frac{8\pi}{9}\,F_0. \tag{11}$$

We measure the depinning force per colloid in realistic many-colloid calculations by comparison with this elementary barrier.

With the adopted parameters, the balance of the Gaussian confinement and the repulsive colloid-colloid repulsion leads in the absence of corrugation ($U_0 = 0$) to an equilibrium spacing $a_{\rm eq} = 0.983$ at the center of the sample, and an overall average density compatible with nearest-neighbor separation $a_{\rm coll} = 1$, which we take as our reference unit distance. It is convenient to define an appropriate length ratio $\rho = a_{\rm las}/a_{\rm coll}$, such that when $\rho = 1$ a fully matched configuration is realized.

## II. THE SIMULATION PROTOCOL

The initial configuration is obtained by cutting a circular island out of a perfect 2D triangular lattice with spacing $a_{\rm coll} = 1$. A simulation is first run with zero external force $F = 0$, in the presence of the confining Gaussian and of the periodic potential of lattice spacing $a_{\rm las}$, simultaneously turned on. Colloid-potential mismatched geometries are generated by taking $a_{\rm las} = 1.05$ (overdense colloids, with solitons) or $a_{\rm las} = 0.95$ (underdense colloids, with antisolitons). In these mismatched cases, still at $F = 0$, the colloid structure in fact relaxes forming lattice matched regions separated by a hexagonal network of soliton/antisoliton regions where the misfit accumulates, in the form of a shorter/longer average colloid-colloid separation, as shown in Fig. 4 and in Fig. 2 respectively. The high mobility of these soliton defects allows the colloidal system to heal most of initial tensile strain of the circular island, thus compressing to an average nearest-neighbor spacing $a_{\rm coll} \simeq a_{\rm eq}$. as the figures show, this leads to a visibly smaller spacing of solitons than antisolitons. In between these overdense and underdense cases, by taking $a_{\rm las} = 1$, we simulate a nominally commensurate case, as in experiment [1]. As illustrated by the $a_{\rm las} = 1$ point of Fig. 5 of the paper, the matched configuration is energetically favorable, with all colloids sitting near to a $W$ potential minimum, and undergoing little or no initial rearrangement during the initial $F = 0$ simulation. Actually, because the island center equilibrium spacing $a_{\rm eq} = 0.983$ is smaller than $a_{\rm las} = 1$ there is still, in this nominally commensurate case, an overall tensile strain. On account of a strong "epitaxial" effect of the periodic potential, this strain is however too weak to give rise to the formation of antisolitons, and is left unhealed in the equilibrated island, that remains fully commensurate. Only under sliding, when soliton structures move in from the edge boundary and sweep across the central region under the action of the dragging force, does the tensile strain have a chance to heal out, giving rise in the very same system that was commensurate at rest to a sparse but regular and nonzero soliton density in the running state. This sliding induced soliton proliferation in statically commensurate colloids agrees very well with what has been reported experimentally. [1]

Mimicking experiment, we introduce an $\hat{\mathbf{x}}$-directed force $F$ acting on each particle, as in Eq. (1). This force is kept fixed for a finite time $t_F$, after which its sign is reversed for the same time duration. After that, this two-step process is repeated with an increased force magnitude $F + \Delta F$. In experiment, the force is produced by the viscous drag of the colloids produced by a fixed-amplitude reciprocating motion of the experimental cell. To mimic this scheme, we carry out each forward and backward run for an amount of time $t_F$ inversely proportional to the force value $F$ itself, and thus the cell speed. The product of $F\,t_F$ is selected in such a way that, under the action of $F$ for a time $t_F$, an isolated unconfined particle would move by a few lattice spacings $F\,t_F/\eta \approx (2 \div 3) a_{\rm las}$ typically, corresponding to at most 3 solitons/antisolitons crossing a given $\hat{\mathbf{y}}$-directed line during a simulation.

As explained above, only the central part of our simulated island is meaningful. Focusing on that region and thus excluding undesired edge effects, we select a square central region of size $80 \times 80$, containing $\sim 7400$ colloids. We drop an initial transient of approximately 30% of the simulation time, and average the $\hat{\mathbf{x}}$-component of the velocity of this central block over the rest of the simulation. This procedure defines the quantity $\langle v_{\rm cm} \rangle$ of Fig. 1c of the paper.

## III. STATIC CONFIGURATIONS

Figures 2-4 show three overall views of the static fully relaxed $F = 0$ configurations for different values of $a_{\rm coll}$, $\rho$. These pictures represent the lowest-energy configurations of the three regions in the phase diagram – Figure 5 in the paper. Soliton/antisoliton patterns are highlighted by coloring colloids differently for different positions relative to the potential profile of Fig. 1: dark, bolder colloids occupy locally unfavorable repulsive regions for the corrugation profile $W$.

Figure 5 illustrates the antisoliton pattern for larger amplitude of the corrugation $U_0$, to be compared with Fig. 2. Note the narrower antisoliton lines, which form the same pattern in the two figures.

Finally, Fig. 6 is to be compared with Fig. 2 to appreciate the effect of the random thermal motions characteristic of 300 K: (i) Brownian fluctuations smear the boundaries between in-registry and antisolitonic regions and (ii) a small thermal expansion is marked by a reduction in $\rho$, and therefore in the separation between antisolitons.

[1] Bohlein T, Mikhael J, Bechinger C (2012) Observation of kinks and antikinks in colloidal monolayers driven across ordered surfaces. Nature Mater 11:126-130.

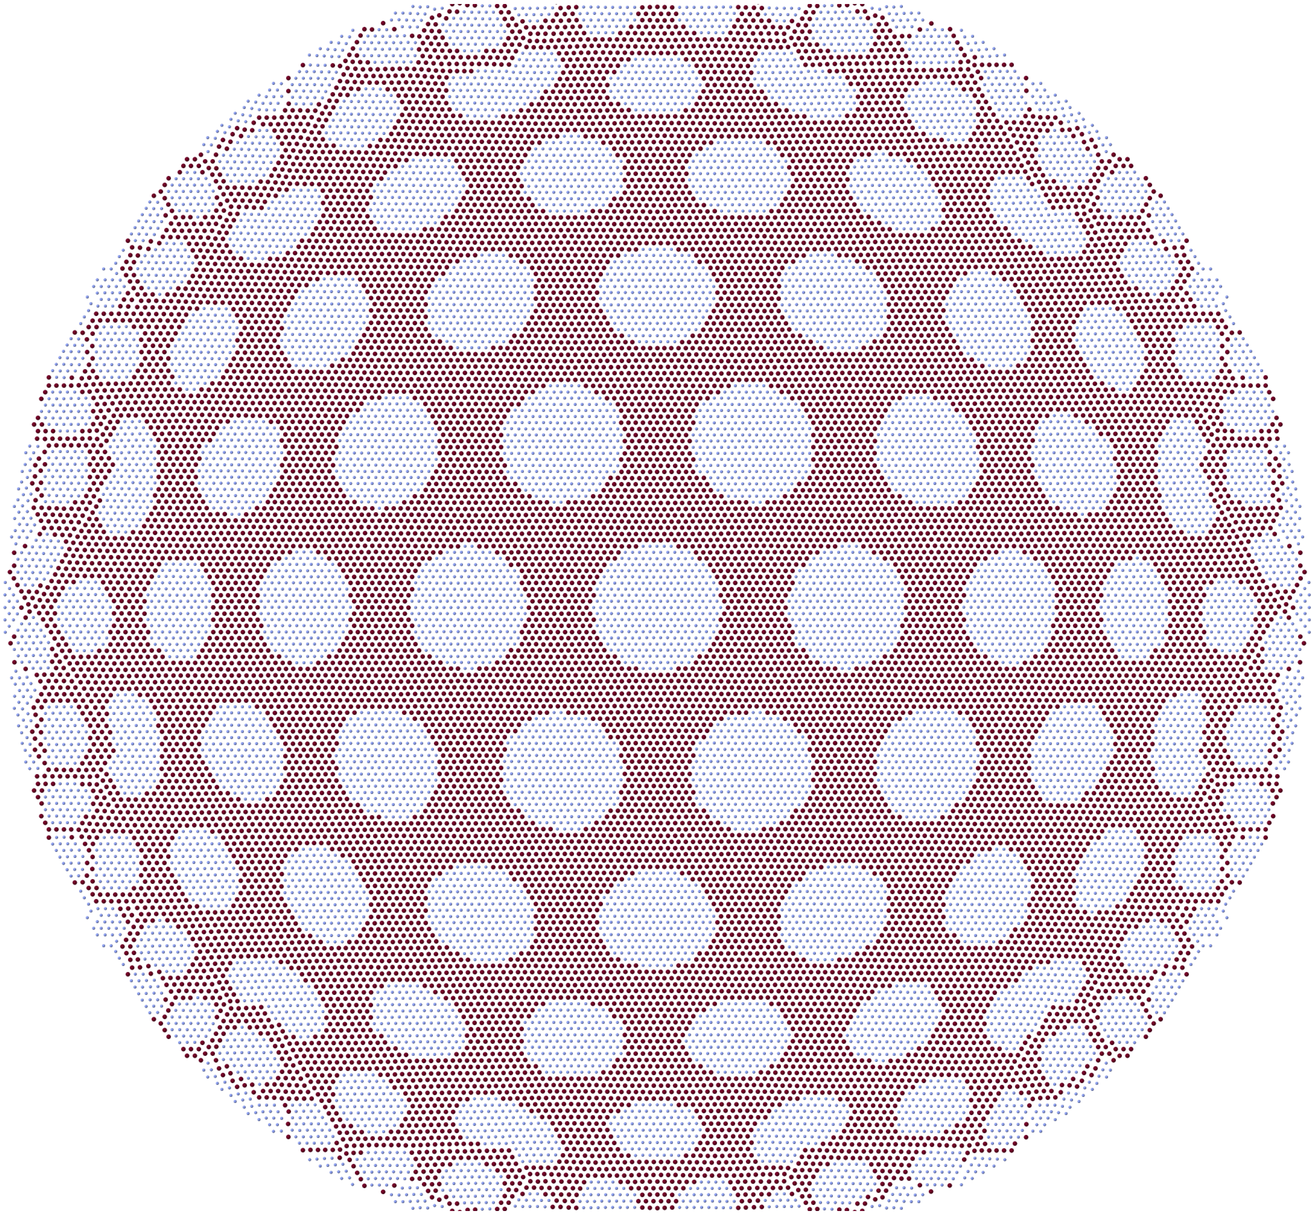

FIG. 2: The static initial configuration for $U_0 = 0.1$, $F = 0$, $a_{\rm las} = 0.95$, i.e. $\rho = 0.95$ (antisoliton incommensurate pattern: AI). Darker dots indicate colloidal particles sitting at a repulsive point of the corrugation landscape, namely with $W(\mathbf{r}) > -U_0/2$. This configuration is essentially unique, since an extremely similar configuration is retrieved at the end of a long relaxation, regardless of the initial condition. The central portion of this figure is represented in Fig. 1b of the paper.


[2] Korda PT, Spalding GC, Grier DG (2002) Evolution of a colloidal critical state in an optical pinning potential landscape. Phys Rev B 66:024504.

[3] Ablowitz MJ, Ilan B, Schonbrun E, Piestun R (2006) Solitons in two-dimensional lattices possessing defects, dislocations, and quasicrystal structures. Phys Rev E 74:035601.

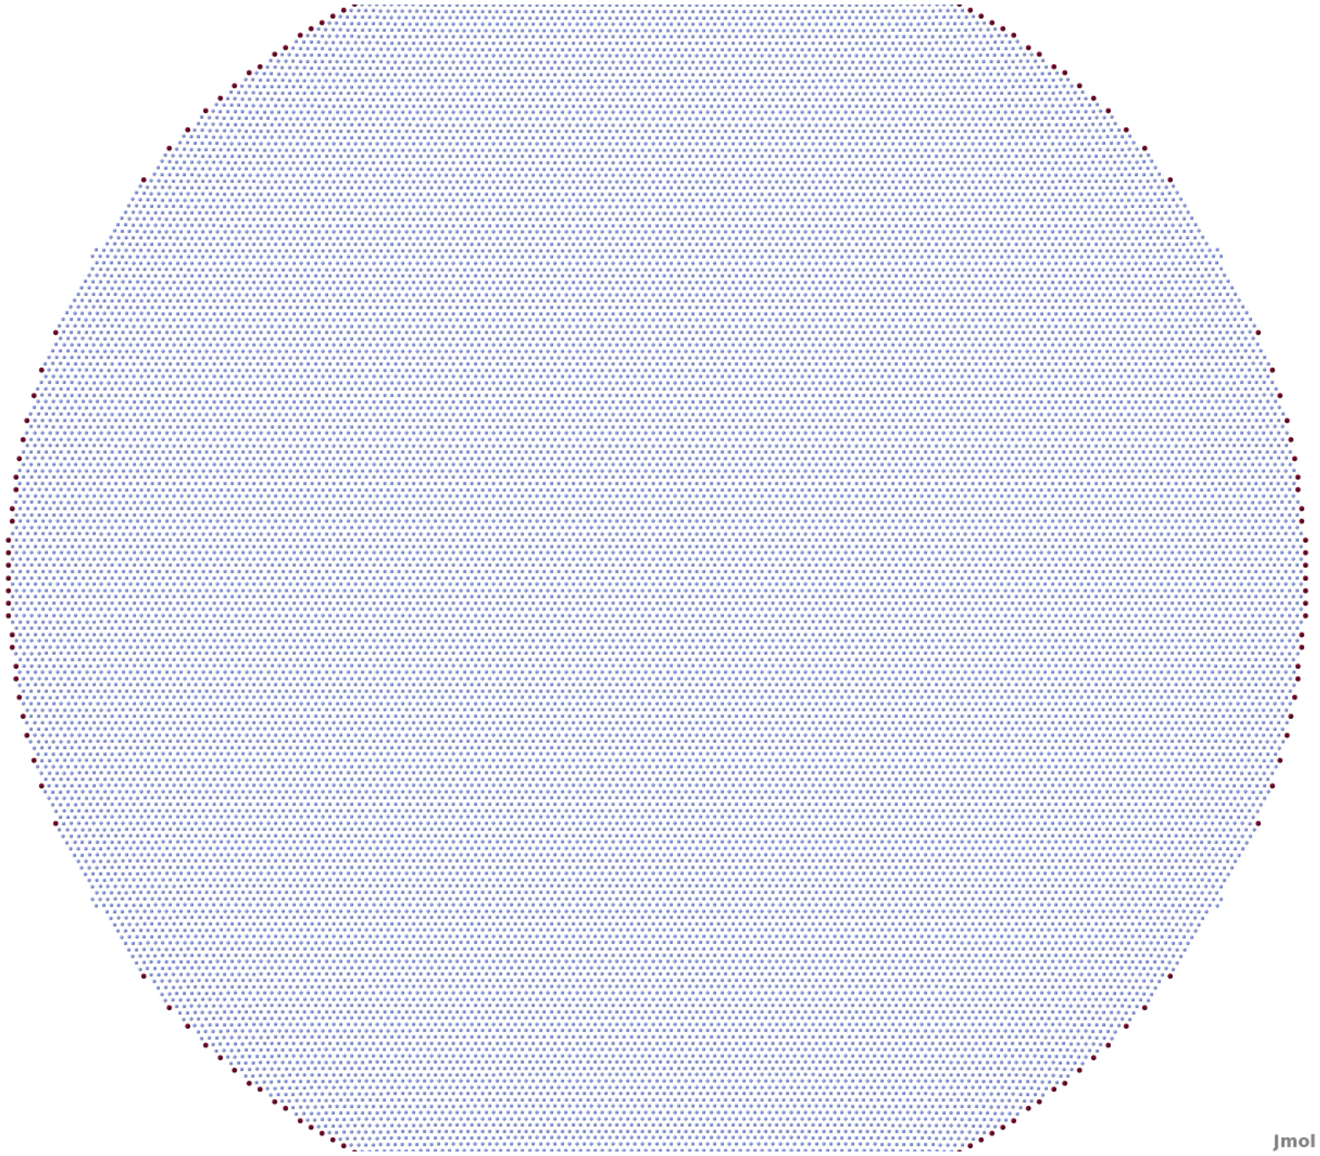


FIG. 3: The static initial configuration for $U_0 = 0.1$, $F = 0$, $a_{\rm las} = 1.00$, i.e. $\rho = 1.02$ (commensurate: CO). Darker dots have the same significance as in Fig. 2. This configuration is the lowest energy state, on the blue-circle curve in the phase diagram – Figure 5 in the paper. The metastable high-energy state of the red-square curve is qualitatively similar to that of the next Fig. 4.

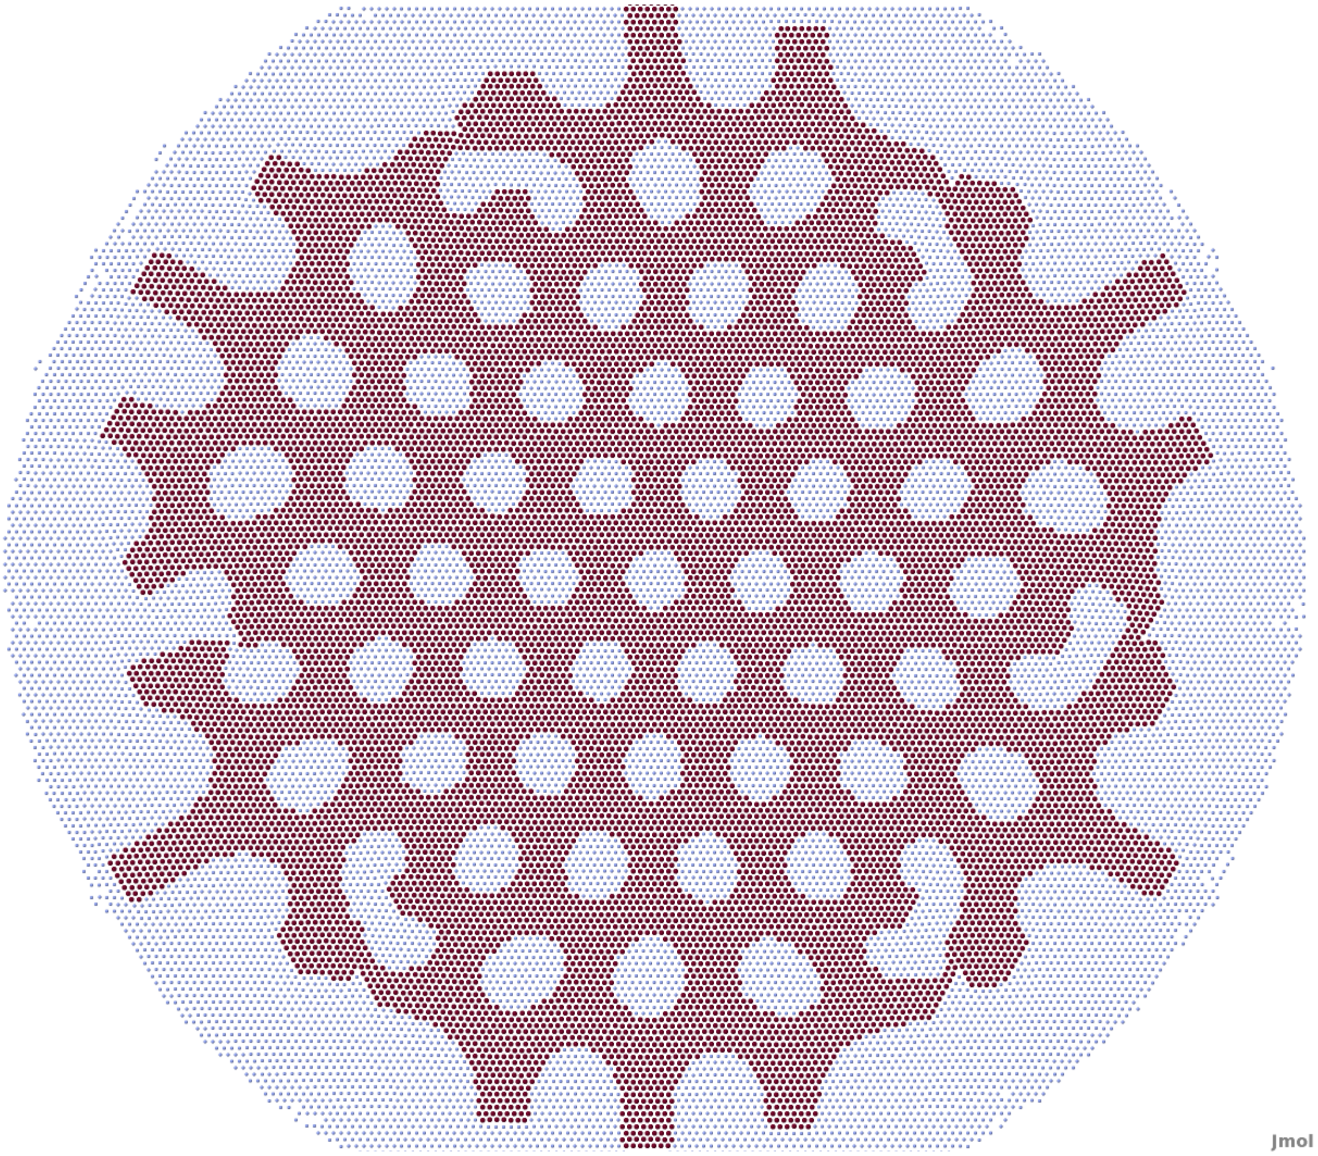


FIG. 4: The static initial configuration for $U_0 = 0.1$, $F = 0$, $a_{\rm las} = 1.05$, i.e. $\rho = 1.05$ (soliton incommensurate pattern: SI). Darker dots have the same significance as in Fig. 2. This configuration is the lowest energy state, on the red-square curve in the phase diagram – Figure 5 in the paper. The metastable high-energy state of the blue-circle curve looks very similar to the one represented in the previous Fig. 3.

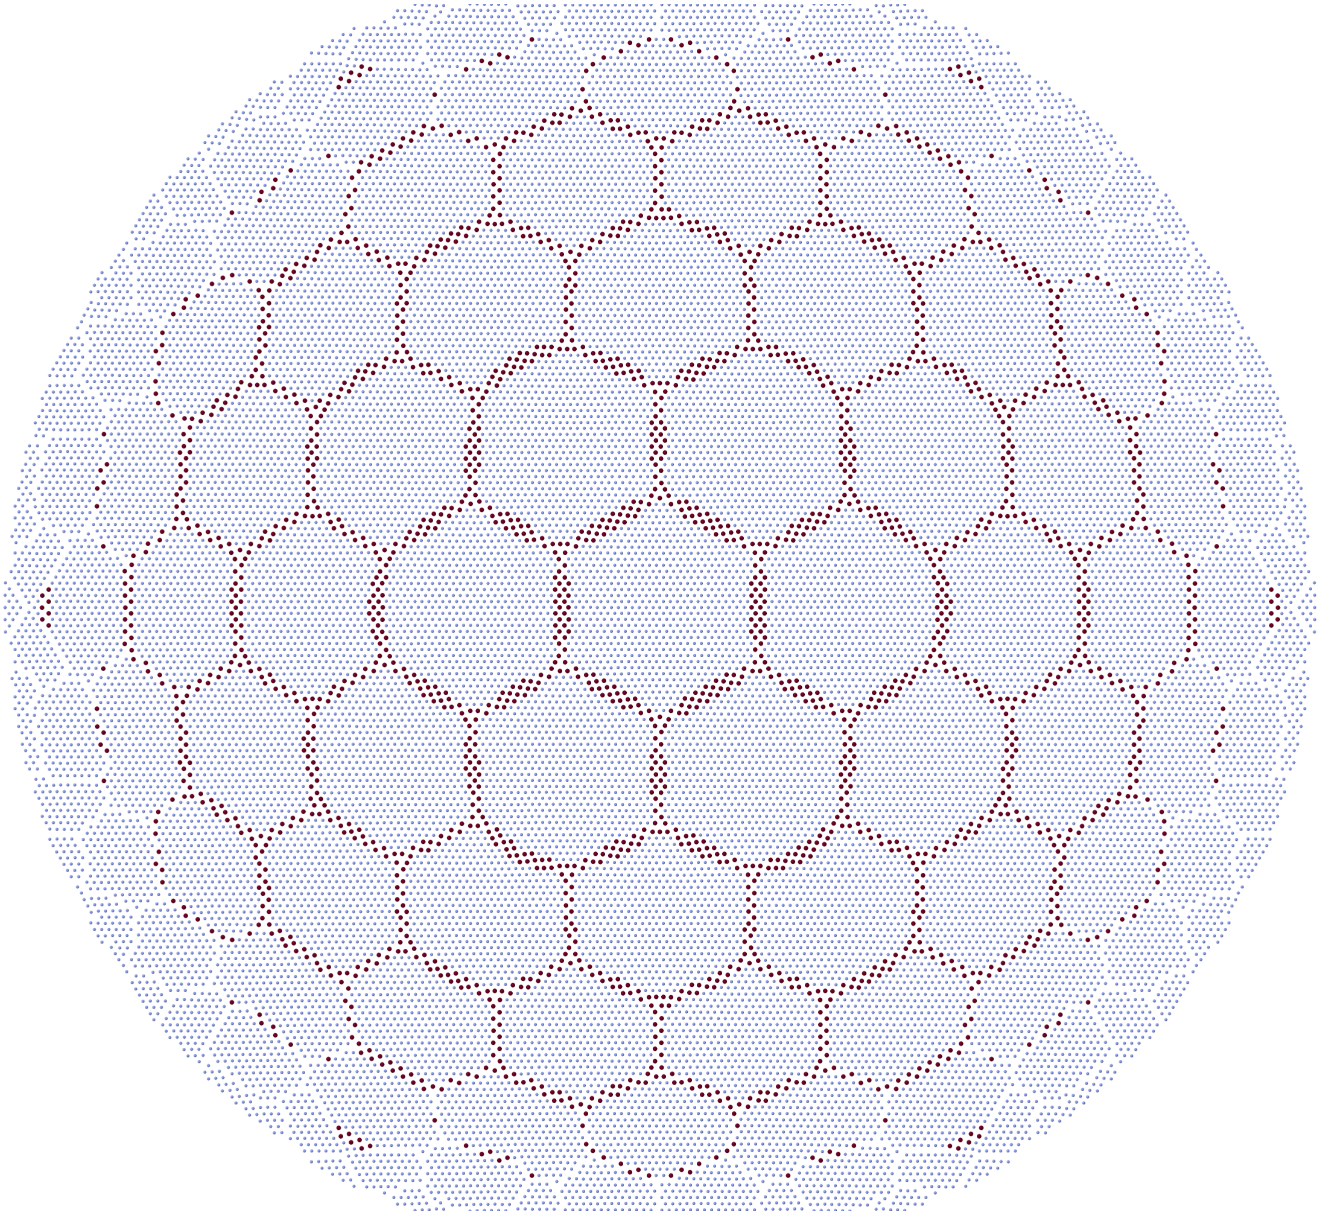

FIG. 5: A typical initial configuration for a stronger ($U_0 = 0.5$) corrugation potential. The other parameters ($F = 0$, $a_{\rm las} = 0.95$, AI) and the color notation are the same as in Fig. 2. By comparison with the weaker corrugation, here antisolitons are much narrower, intersecting and isolating well-faceted in-registry regions. Note that the pattern formed by the center of the antisoliton lines is the same in both figures.

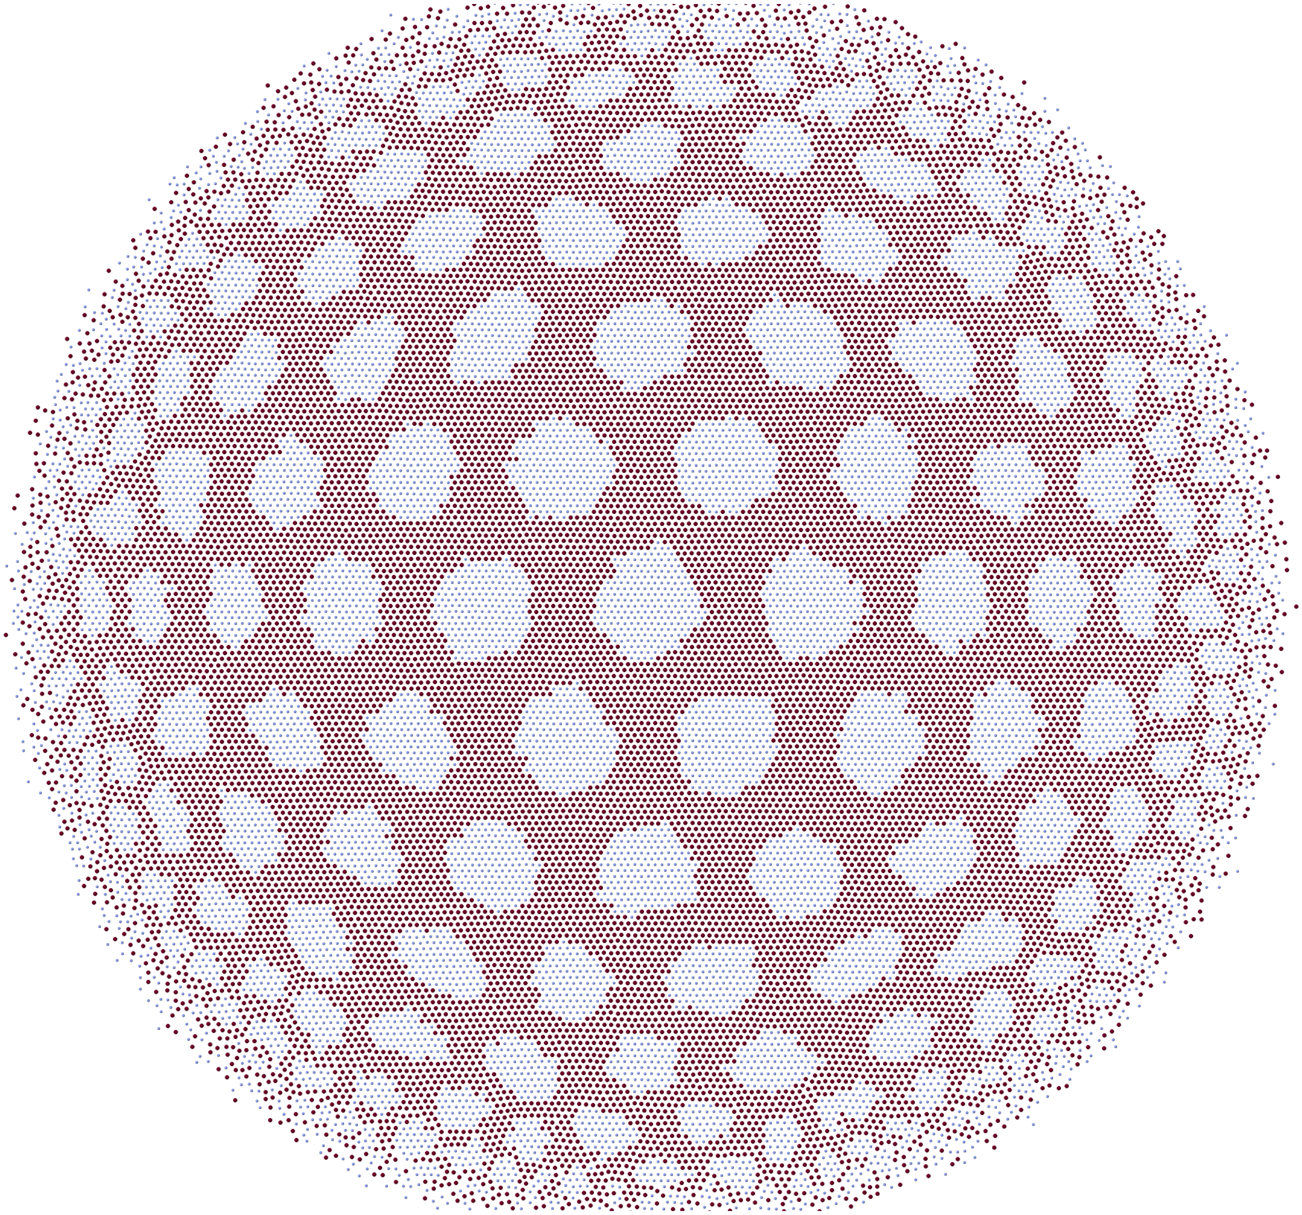

FIG. 6: Effect of thermal fluctuations. A typical $F = 0$ snapshot of a Langevin simulation at $k_\mathrm{B}T = 0.04$, corresponding to room temperature in model units. The parameters ($U_0 = 0.1$, $F = 0$, $a_\mathrm{las} = 0.95$, AI) and the color notation are the same as in Fig. 2. By comparison with the $T = 0$ configuration, the antisoliton pattern is only marginally affected by thermal noise. A minor thermal expansion is responsible for a slight reduction of $\rho$, with a correspondingly denser antisolitonic pattern.
